# Supplementary material for: EHRXQA: A Multi-Modal Question Answering Dataset for Electronic Health Records with Chest X-ray Images
Source: arXiv:2310.18652 source file (2023-12-25)
Supplement: Supplementary file 2 [file vqa_exp_template.tex]

\begin{table}[H]
    \setlength{\tabcolsep}{3pt}
    \noindent
    \centering
        \captionsetup{font={small}}
        \caption{Comparison of performance of models on \textbf{MIMIC-CXR-VQA (\textit{Template})}. 
        }
        \resizebox{0.4\linewidth}{!}{%
            \begin{tabular}{@{}cccccc@{}}
            \toprule
            \multirow{2}{*}{Model} & \multicolumn{2}{c}{Valid} & \multicolumn{2}{c}{Test} \\ \cmidrule(l){2-5}
                                   & Acc & F1 (micro) & Acc & F1 (micro) 
                                   \\ \midrule
            Prior (Most)
            & 26.8
            & 0.27
            & 25.3
            & 0.25 \\
            Prior (Question)
            & 34.2
            & 0.34
            & 32.4
            & 0.32 \\
            PubMedCLIP
            & $53.6_{\text{ ± } 1.0}$ 
            & $0.58_{\text{ ± } 0.01}$ 
            & $53.2_{\text{ ± } 0.1}$ 
            & $0.57_{\text{ ± } 0.01}$ \\
            PubMedCLIP$^{\ast}$
            & $53.6_{\text{ ± } 0.8}$ 
            & $0.57_{\text{ ± } 0.01}$ 
            & $53.4_{\text{ ± } 0.6}$ 
            & $0.57_{\text{ ± } 0.01}$ \\
            MedViLL$^{\ast}$
            & $65.9_{\text{ ± } 0.2}$ 
            & $0.70_{\text{ ± } 0.00}$ 
            & $65.4_{\text{ ± } 0.3}$ 
            & $0.68_{\text{ ± } 0.00}$ \\
            M$^{3}$AE
            & $69.7_{\text{ ± } 0.2}$ 
            & $0.73_{\text{ ± } 0.00}$ 
            & $69.1_{\text{ ± } 0.3}$ 
            & $0.72_{\text{ ± } 0.00}$ \\
            M$^{3}$AE$^{\ast}$
            & $70.7_{\text{ ± } 0.3}$ 
            & $0.74_{\text{ ± } 0.00}$ 
            & $69.7_{\text{ ± } 0.4}$ 
            & $0.73_{\text{ ± } 0.00}$ \\
            \bottomrule
            \end{tabular}%
            }
  \end{table}
