# Supplementary material for: EHRXQA: A Multi-Modal Question Answering Dataset for Electronic Health Records with Chest X-ray Images
Source: arXiv:2310.18652 source file (2023-12-25)
Supplement: Supplementary file 3 [file vqa_exp_template_content.tex]

\begin{table}[H]
\setlength{\tabcolsep}{3pt}
    \noindent
    \centering
    \caption{ Comparison of performance (Acc) of models across content types on \textbf{MIMIC-CXR-VQA (\textit{Template})}.}
    \resizebox{0.75\textwidth}{!}{%
        \begin{tabular}{cccccccc}
        \toprule
        \multicolumn{8}{c}{Valid} \\
        \midrule
        Model & Plane & Gender & Size & Abnormality & Anatomy & Attribute & Condition \\
        \midrule
        Prior (Most) 
        & $16.7 $ 
        & $16.7 $ 
        & $50.0 $ 
        & $24.7 $ 
        & $0.0 $ 
        & $0.0 $ 
        & $50.0 $ \\
        Prior (Question) 
        & $50.0 $ 
        & $50.0 $ 
        & $50.0 $ 
        & $29.5 $ 
        & $10.9 $ 
        & $16.9 $ 
        & $50.0 $ \\
        PubMedCLIP 
        & $62.8_{\text{ ± } 0.7}$ 
        & $42.9_{\text{ ± } 1.2}$ 
        & $77.7_{\text{ ± } 0.6}$ 
        & $49.8_{\text{ ± } 0.6}$ 
        & $31.7_{\text{ ± } 1.1}$ 
        & $35.5_{\text{ ± } 0.4}$ 
        & $70.8_{\text{ ± } 0.6}$ \\
        PubMedCLIP$^\ast$ 
        & $61.9_{\text{ ± } 0.7}$ 
        & $43.9_{\text{ ± } 1.1}$ 
        & $77.7_{\text{ ± } 1.1}$ 
        & $50.1_{\text{ ± } 0.4}$ 
        & $32.0_{\text{ ± } 0.5}$ 
        & $35.7_{\text{ ± } 0.2}$ 
        & $70.9_{\text{ ± } 0.3}$ \\
        MedViLL$^\ast$ 
        & $99.0_{\text{ ± } 0.1}$
        & $91.0_{\text{ ± } 0.2}$
        & $76.3_{\text{ ± } 0.5}$
        & $60.4_{\text{ ± } 0.3}$
        & $44.4_{\text{ ± } 0.4}$
        & $56.1_{\text{ ± } 0.1}$
        & $76.7_{\text{ ± } 0.4}$ \\
        M$^{3}$AE 
        & $99.3_{\text{ ± } 0.1}$
        & $94.6_{\text{ ± } 0.3}$
        & $81.7_{\text{ ± } 0.3}$
        & $65.1_{\text{ ± } 0.1}$
        & $48.5_{\text{ ± } 0.1}$
        & $60.8_{\text{ ± } 0.3}$
        & $79.4_{\text{ ± } 0.4}$ \\
        M$^{3}$AE$^\ast$
        & $99.4_{\text{ ± } 0.3}$
        & $93.9_{\text{ ± } 0.5}$
        & $81.9_{\text{ ± } 0.6}$
        & $66.4_{\text{ ± } 0.3}$
        & $50.1_{\text{ ± } 0.5}$
        & $61.9_{\text{ ± } 0.7}$
        & $80.3_{\text{ ± } 0.1}$ \\
        \toprule
        \multicolumn{8}{c}{Test} \\
        \midrule
        Model & Plane & Gender & Size & Abnormality & Anatomy & Attribute & Condition \\
        \midrule
        Prior (Most)
        & $17.1 $ & $16.7 $ & $43.3 $ & $23.9 $ & $0.0 $ & $0.0 $ & $50.4 $ \\
        Prior (Question) 
        & $48.7 $ 
        & $50.0 $
        & $43.3 $ 
        & $28.8 $ 
        & $10.9 $ 
        & $13.1 $ 
        & $50.4 $ \\
        PubMedCLIP
        & $61.3_{\text{ ± } 1.3}$
        & $43.9_{\text{ ± } 0.6}$
        & $75.5_{\text{ ± } 1.1}$
        & $47.7_{\text{ ± } 0.2}$
        & $34.0_{\text{ ± } 1.7}$
        & $35.6_{\text{ ± } 0.5}$
        & $71.4_{\text{ ± } 0.4}$ \\
        PubMedCLIP$^\ast$ 
        & $60.5_{\text{ ± } 1.5}$
        & $44.0_{\text{ ± } 3.2}$
        & $76.2_{\text{ ± } 1.0}$
        & $47.7_{\text{ ± } 0.5}$
        & $34.4_{\text{ ± } 0.8}$
        & $35.8_{\text{ ± } 0.3}$
        & $71.1_{\text{ ± } 1.0}$ \\
        MedViLL$^\ast$ 
        & $99.5_{\text{ ± } 0.3}$
        & $92.0_{\text{ ± } 0.1}$
        & $75.0_{\text{ ± } 0.9}$
        & $60.8_{\text{ ± } 0.2}$
        & $46.7_{\text{ ± } 0.5}$
        & $54.9_{\text{ ± } 0.4}$
        & $76.0_{\text{ ± } 0.3}$ \\
        M$^{3}$AE 
        & $99.1_{\text{ ± } 0.1}$
        & $94.5_{\text{ ± } 0.1}$
        & $81.1_{\text{ ± } 0.5}$
        & $64.2_{\text{ ± } 0.1}$
        & $51.1_{\text{ ± } 0.3}$
        & $60.5_{\text{ ± } 1.1}$
        & $78.6_{\text{ ± } 0.1}$ \\
        M$^{3}$AE$^\ast$ 
        & $99.5_{\text{ ± } 0.3}$
        & $93.3_{\text{ ± } 1.0}$
        & $80.3_{\text{ ± } 1.2}$
        & $65.1_{\text{ ± } 0.2}$
        & $53.2_{\text{ ± } 1.3}$
        & $60.8_{\text{ ± } 0.8}$
        & $78.9_{\text{ ± } 0.3}$ \\
        \bottomrule
    \end{tabular}
    }
\end{table}
